# Supplementary material for: Tactile-Filter: Interactive Tactile Perception for Part Mating
Source: arXiv:2303.06034 source file (2023-06-05)
Supplement: Supplementary file 1 [file appendix.tex]

\clearpage
\onecolumn
\appendix
\subsection{Additional Results}

\subsubsection{Updates of belief maps from interactions}
To facilitate the understanding of how \textit{Tactile-Filter} updates its belief through interactions, we conducted an experiment using the \textit{MLTF} board, which features letters ``M'', ``L'', ``T'',  and ``F'' as presented in \fref{fig:pipeline} (leftmost picture). The visualizations generated from this experiment as shown in \fref{fig:mltf_visualizations} demonstrate that our method successfully narrows down the distribution of the hole's initial contact pose and its corresponding hole types.
